# Supplementary material for: Investigating Pretrained Language Models for Graph-to-Text Generation
Source: arXiv:2007.08426 source file (2021-09-27)
Supplement: Supplementary file 1 [file additionalresults.tex]

% \begin{table}
% \centering
% {\renewcommand{\arraystretch}{0.8}

% \caption{Statistics for the graph-to-text benchmarks.}
% \label{tab:datastatistics}
% \end{table}

% \begin{table*}[t]
% \centering
% \resizebox{\textwidth}{!}{  
% \begin{tabular}{@{\hspace*{3mm}}l@{\hspace*{2mm}}r@{\hspace*{3mm}}r@{\hspace*{2mm}}r@{\hspace*{2mm}}r@{\hspace*{3mm}}}  
% \toprule
%  & \textbf{AMR17} & \textbf{WebNLG} & \textbf{AGENDA}  \\
% \midrule
% \#Train & 36,521 & 18,102 & 38,720  \\
% \#Dev & 1,368 & 872 & 1,000  \\
% \#Test & 1,371 & 1,862 & 1,000 \\
% \midrule
% \#Relations & 155 & 373 & 7 \\
% Avg \#Nodes & 15.63 & 4.0 & 13.4 \\
% \midrule
% Avg \#Tokens & 16.1 & 31.5 & 157.9 \\
% %Vocabulary size & - & 373 & 7 \\
% %SR11 & 18,102 & 872 & 971 & 373  \\

% \bottomrule
% \end{tabular}
% \caption{Statistics for the graph-to-text benchmarks.}
% \quad
% \begin{tabular}{l|ll}
% \toprule
% %  \multirow{3}{*}{\rotatebox{90}{\textsc{CompSc}}} 
% \cs   
%  &  \arccite                   
%  & \sciie \\
% %\cmidrule{2-4}  
% \midrule
% \tapt
% & 67.4$_{1.8}$                
% & 79.3$_{1.5}$ \\
% Transfer-\tapt 
% & 64.1$_{2.7}$ ($\downarrow$3.3) 
% & 79.1$_{2.5}$ ($\downarrow$0.2) \\
% \bottomrule
% \toprule
% % \multirow{3}{*}{\rotatebox{90}{\textsc{reviews}}} 
% \reviews    
% &  \helpful                         
% & \imdb     \\
% %\cmidrule{2-4} 
% \midrule
% \tapt    
% & 68.5$_{1.9}$ 
% & 95.7$_{0.1}$\\
%  Transfer-\tapt 
% & 65.0$_{2.6}$ ($\downarrow$3.5)    
% & 95.0$_{0.1}$ ($\downarrow$0.7) \\
% \bottomrule
% \end{tabular}}
% \caption{Statistics for the graph-to-text benchmarks.}
% \label{tab:transfer_test_results}
% \end{table*}

\begin{table*}[t]
\begin{tabularx}{\linewidth}{CC}
{
\begin{tabular}{@{\hspace*{1mm}}l@{\hspace*{1mm}}c@{\hspace*{2mm}}c@{\hspace*{2mm}}c@{\hspace*{1mm}}}  
\toprule
\textbf{Model} & \textbf{chrF++} & \textbf{BS (F1)} & \textbf{MS}  \\
\midrule
%\citet{damonte-cohen-2019-structural} & 23.30 & - & 50.40 & - & - & - \\
\citet{dcgcnforgraph2seq19guo} & 57.30 & - & - \\
\citet{ribeiro-etal-2019-enhancing}  & - & - & - \\
\citet{zhu-etal-2019-modeling} & 64.05 & - & - \\
\citet{cai-lam-2020-graph} & 59.40 & - & - \\
\citet{zhao-etal-2020-line} &  - & - & - \\
\citet{doi:10.116200297} &  65.80 & - & - \\
\citet{yao-etal-2020-heterogeneous}  &  65.60 & - & - \\
\midrule
\small{\textit{based on PLMs}}  &  \\[.2em]
\citet{mager2020gpttoo}  & 63.89  & -& - \\
\citet{harkous2020text}  &  -  & - & - \\
\midrule
BART\textsubscript{base}  &  66.65 & 95.22 & 60.78  \\
BART\textsubscript{large}  & 71.06 & 96.08 & 65.74  \\
%\midrule
T5\textsubscript{small} &  68.78 & 95.62 & 63.70  \\
T5\textsubscript{base} & 70.81 & 95.99 & 65.63  \\
T5\textsubscript{large} & \textbf{72.57} & \textbf{96.27} & \textbf{67.37} \\
\midrule
\multicolumn{3}{l}{\small{\textit{with task-adaptive pretraining}}}  \\[.2em]
BART\textsubscript{large} + \textsc{lma} & 71.14 & 95.94 & 64.75  \\
T5\textsubscript{large} + \textsc{lma} & 72.83 & 96.32 & 67.44  \\[.7em]
BART\textsubscript{large} + \textsc{sta} \small{\textsc{(200K)}} & 72.26 & 96.21 &66.75 \\
BART\textsubscript{large} + \textsc{sta} \small{\textsc{(2M)}} & 73.58 & 96.43 & 68.14 \\
T5\textsubscript{large} + \textsc{sta} \small{\textsc{(200K)}} & 74.09 & 96.51 & 68.86 \\
T5\textsubscript{large} + \textsc{sta} \small{\textsc{(2M)}} & \textbf{\textit{74.79}} & \textbf{\textit{96.59}} & \textbf{\textit{69.53}} \\
\bottomrule
\end{tabular}}
\caption{Results of the chrF++, BertScore (BS) and MoverScore (MS) scores for the LDC2017T10 test set. \textbf{Bold} (\textbf{\textit{Italic}}) indicates the best score without (with) task-adaptive pretraining.}
\label{tab:results-amr-appendix}
&
{
\begin{tabular}{@{\hspace*{1mm}}l@{\hspace*{1mm}}ccc@{\hspace*{1mm}}}  
\toprule
\textbf{Model} & \textbf{chrF++} & \textbf{BS (F1)} & \textbf{MS}  \\
\midrule
\citet{schmitt2020modeling} & 44.53 & -& -\\
\citet{ribeiro-etal-2020-modeling} & 46.37 & -& - \\
\midrule
BART\textsubscript{base} & 48.02 & 89.36 & 34.33 \\
BART\textsubscript{large} & \textbf{50.44} & 88.74 & 32.24 \\
T5\textsubscript{small}  & 44.91 & 88.56 & 30.25 \\
T5\textsubscript{base} & 48.14 &  88.81 & 31.33 \\
T5\textsubscript{large} &  48.14 & \textbf{89.60} & \textbf{35.23} \\
\midrule
\multicolumn{2}{l}{\small{\textit{with task-adaptive pretraining}}}  \\[.2em]
BART\textsubscript{large} + \textsc{lma} & 51.33 & 89.12 & 33.42 \\
T5\textsubscript{large} + \textsc{lma} & 49.37 & 89.75 & 36.13 \\[.7em]
BART\textsubscript{large} + \textsc{sta} & \textbf{\textit{51.63}} & 89.27 & 34.28 \\
T5\textsubscript{large} + \textsc{sta} & 50.27 & \textbf{\textit{89.93}} & \textbf{\textit{36.86}} \\
%\midrule
%BART\textsubscript{large} + \textsc{STA}\textsubscript{WebNLG} & 25.28 & 25.68 & 51.34 & 89.34 & 34.70 & -11.06 \\
\bottomrule
\end{tabular}}
\caption{Results of the chrF++, BertScore (BS) and MoverScore (MS) scores for AGENDA test set. \textbf{Bold} (\textbf{\textit{Italic}}) indicates best scores without (with) task-adaptive pretraining.}
\label{tab:results-agenda-appendix}
\end{tabularx}
\end{table*}
